# Supplementary material for: Localization with Sampling-Argmax
Source: arXiv:2110.08825 source file (2021-10-17)
Supplement: Supplementary file 1 [file experiment.tex]

\section{Correlation Testing}
\label{sec:corr}

\begin{table}[ht]
    \vspace{-5mm}
    \caption{Correlation testing on MTFL.}
    \label{tab:corr}
    \centering
    \begin{tabular}{lcc}
        \toprule
        Method & Corr. (Abs) &  Corr. (Rel) \\
        \midrule
        Soft & -0.261 & -0.270 \\
        Soft w/ V.R & -0.267 & -0.282 \\
        Soft w/ D.R & -0.263 & -0.279 \\
        \midrule
        Samp. Uni. & -0.263 & -0.276 \\
        Samp. Tri. & -0.278 & -0.301 \\
        Samp. Gau. & \textbf{-0.327} & \textbf{-0.355} \\
        \bottomrule
    \end{tabular}
\end{table}
